# Supplementary material for: The mechanism of the irradiation synergistic effect of Silicon bipolar junction transistors explained by multiscale simulations of Monte Carlo and excited-state first-principle calculations
Source: arXiv:2305.16601 source file (2023-07-18)
Supplement: Supplementary file 1 [file supplemental.pdf]

# Supplemental material for "The mechanism of the Silicon irradiation synergistic effect explained by multiscale simulations of Monte Carlo and excited-state first-principle calculations"


Zeng-hui Yang,[1,2] Yang Liu,[1,2] Ning An,[1,2] and Xingyu Chen[1,2]

[1] *Microsystem and Terahertz research center, China Academy of Engineering Physics, Chengdu, China 610200*
[2] *Institute of Electronic Engineering, China Academy of Engineering Physics, Mianyang, China 621000*



(Dated: June 26, 2023)



This supplemental material contains the discussion of the convergence problem of ΔSCF and Vineyard prefactor, the discussion of the applicability and accuracy of Geant4 simulations, the estimation of the reaction rate constant according to the parameters of the defect-based model, and the technical details of calculations.


## I. CONVERGENCE PROBLEM OF ΔSCF

We encounter severe convergence problem in ΔSCF calculations when using the default smearing of VASP (0.05). By plotting the energy of each SCF step for the diverging calculations, we can see that two or more electronic states are involved. This is typical variational collapse behavior. Only occupied orbitals are variationally optimized in the SCF loop, whose orbital energies would decrease in the process. In ΔSCF, however, the occupied orbitals are not the ones with the lowest energies. Therefore the energy of some occupied orbital may go below an unoccupied orbital in an SCF step and become unoccupied in the next step. This problem is inherent to Born-Oppenheimer approximations, indicating near degeneracies at the current geometry, which might be close to an avoided crossing in excited state. There are some existing methods[1–3] that are able to suppress the oscillation between states, but they require extensive modification to the SCF code.

For simplicity, we attempt to achieve convergence of ΔSCF by tuning the input parameters in this work. A small density mixing parameter sometimes leads to convergence, but the performance is inconsistent. We find that a large smearing parameter is usually enough for neutral systems to converge, but charged systems still diverge in many cases. The effect of a large smearing parameter is that the occupation numbers change slowly from occupied to unoccupied near the Fermi level. In ΔSCF, all the orbitals in between $E_F^{(1)}$ and $E_{F,0}$ (see Fig. 2 of the main text) can become partially occupied with a large smearing number, so there is no gap in the variationally optimized orbitals. The oscillation between states is suppressed since the total energy change is continuous even when the ordering of orbitals change during the SCF. We tested the effect of different smearing parameters on $V_2$, and find that the entropy increases rapidly after $\sigma = 0.2$ eV. However, $\sigma = 0.2$ eV cannot guarantee convergence for all systems studied in this work, especially during geometry optimizations. We choose to use $\sigma = 0.3$ eV for all calculations in this work.

The error due to using a large $\sigma$ is small in many cases. For example, both the errors in the total energy of $V_2$ and in $E_a^{\mathrm{mig,gs}}$ of $\mathrm{Si_i}$ are about 0.03 eV. However, the large $\sigma$ can introduce artifacts in the geometry. Fig. 1 shows the NEB curves of $V_2$ dissociation. For the ground state case, the NEB curve develops a spurious local minimum in the middle as $\sigma$ increases. Comparing the ground-state and excited-state curves, the local minimum in the excited-state curve is highly possible to be an artifact as well, even though we cannot obtain converged excited-state results for smaller $\sigma$. We will try to eliminate this problem in future works by employing more sophisticated methods for ΔSCF convergence.

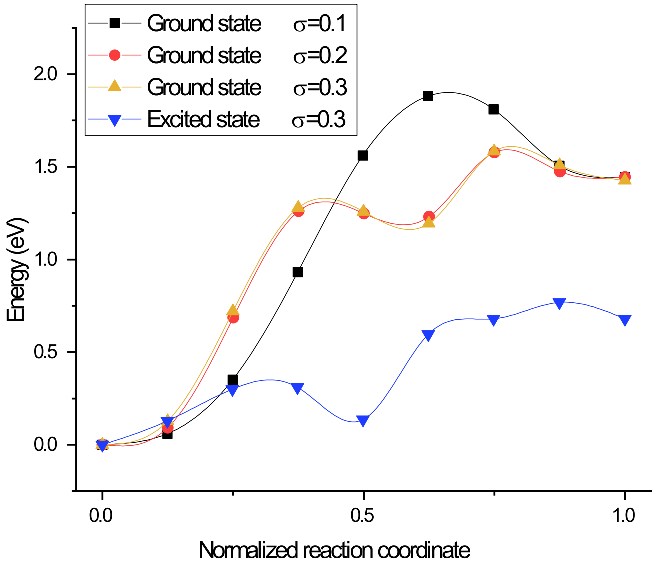


FIG. 1. The NEB curves of $V_2$ dissociation with different smearing parameter. The excited state has 26 excited electrons. Only $\sigma = 0.3$ eV curve is shown for the excited case due to divergence of calculations with smaller $\sigma$.

## II. VINEYARD PREFACTOR CALCULATIONS

The reaction rate of a reaction is determined by the Arrhenius equation $k = A\exp[-E_a/(k_B T)]$, where $A$ is the prefactor, $E_a$ the activation energy, $k_B$ is the Boltzmann constant and $T$ is the temperature. The attempt

frequency is one of the main parts of the prefactor and is often estimated using the Debye frequency in experimental studies.[4] For computational studies, the Vineyard method[5, 6] is widely used to estimate the attempt frequency. The method only depends on the vibration frequencies of the initial geometry and the transition state, which can be calculated easily.

In this work, we used the Vineyard method to estimate the prefactor of diffusivity. However, we find convergence with respect to the degrees of freedoms included in the calculation difficult to achieve. The calculated ground state Vineyard prefactors for the diffusion of $V_2$ and $O_i$ are different to the experimental values[7, 8] by one order of magnitude, and that of V is different to the experimental value[9] by 4 orders of magnitudes. This is probably due to the $3 \times 3 \times 3$ supercell being too small according to Ref. [10], which calculates the Vineyard prefactor in $\alpha$-iron and listed its change with the number of atoms. Ref. [10] shows that about 300 atoms are needed to get a Vineyard prefactor with the correct order of magnitude, and over 2000 atoms are needed to converge the Vineyard prefactor. Because of this problem, we only compare the relative size of the ground-state and excited-state prefactors of $V_2$ diffusion in the main text, where the excited-state (26 electrons) one is about 20 times greater than the ground-state one.

## III. APPLICABILITY AND ACCURACY OF GEANT4 SIMULATIONS

The energy range of Geant4 simulations is usually much higher than that of DFT, so these two methods are rarely used together. In this work, the energy gap between the two methods is mended by the MicroElec low-energy models of Geant4. However, the MicroElec models are only accurate down to a few eV for electrons[11] (even though the models include data of lower energies), so the last few steps of the electron tracks are inaccurate. This inaccuracy is one of the reasons for us not using the electron energy spectrum in DFT calculations. Another reason is that the treatment of electronic structure in the de-excitation models and MicroElec models of Geant4 is simplistic, only concerning the shell structure of atoms, so the electron energy spectrum may be incompatible with the DFT band structure.

Geant4 simulations show that the moving distance of the low-energy (less than a few eV) electrons is at the Angstrom or nm level. This distance is very small for Geant4, but not small for DFT. The low-energy inaccuracy of Geant4 therefore affects the electron distribution as well. In the future, we will implement more accurate models (such as the PENELOPE model[12] which is accurate down to the band gap) in Geant4 and compare the result.

## IV. ESTIMATING THE REACTION RATE CONSTANT FROM FITTING PARAMETERS IN THE DEFECT-BASED MODEL OF THE ISE

Although the functional form of the defect-based ISE model of Silicon BJTs[13] is obtained by solving coupled reaction rate equations, most of the rate constants cannot be calculated from the fitted model parameters, because they becomes inseparable from each other and from certain defect concentrations in the final formula of $I_B$. The reaction $V_2 + O_i \rightarrow V_2O$ in P-type Silicon is the only one whose rate constant $k$ can be deduced from the model parameters. For this reaction, the model assumes that $c_{O_i}$ is constant, so it is absorbed into the rate constant by writing $\kappa = kc_{O_i}$. $\kappa$ is related to the characteristic dose $D_c$ by $\kappa = D_c/R$, where $R$ is the dose rate. $D_c$ is fitted from experimental data, which is 0.26 krad(Si) and 0.38 krad(Si) at $R = 10$ mrad(Si)/s and $R = 10$ rad(Si)/s respectively. Since $c_{O_i}$ is typically about $10^{18}$ cm$^{-3}$[14], we obtain the low- and high-dose-rate estimation of the reaction rate constant as $k^{\text{low}} = 4 \times 10^{-23}$ cm$^3$·s$^{-1}$ and $k^{\text{high}} = 3 \times 10^{-20}$ cm$^3 \cdot s^{-1}$.

This can be explained by the lowing of the migration barrier of $V_2$. Due to high migration activation energies, defect reactions in solids are often diffusion-limited, i.e. the reaction activation energy is much less than the migration activation energy. For reactions with two reactants (denoted as X and Y), the reaction rate at equilibrium is[15, 16]

$$\frac{\partial c_X}{\partial t} = -4\pi R_{X,Y}(D_X + D_Y)c_X c_Y, \tag{1}$$

where $R_{X,Y}$ is the effective reaction distance, and $D_X$ and $D_Y$ are diffusivities of X and Y. The rate constant $k = -4\pi R_{X,Y}(D_X + D_Y)$ is proportional to the sum of diffusivities of reactants, which increase due to the migration activation energies decreasing with more excited electrons. This results in the higher rate constants at higher $\gamma$-ray dose rate.

We also mentioned in the main text the possible connection to the lowing of the formation energy of $V_2$. Considering that the rate constant is obtained by fitting, and the concentration change due to formation energy change is not considered in the previous model[13], the fitting process may incorporate this change into the rate constant, and the rate constant would appear to be higher at higher dose rate.

It should be noted that the dose rate effect is more complicated than it appears. Since the reaction happens very slowly without $\gamma$-ray irradiation, it can be argued that the rate constant with respect to the dose ($k_D = k/R$) is more relevant. We obtain $k_D^{\text{low}} = 4 \times 10^{-21}$ cm$^3$·rad(Si)$^{-1}$ and $k_D^{\text{high}} = 3 \times 10^{-21}$ cm$^3$·rad(Si)$^{-1}$, which shows that the rate constant has a sub-linear relation with the dose rate. Such sub-linear behavior has been observed in other aspects of the dose rate effect as well, and currently there is no comprehensive explanation. Another example of unexplained dose-rate effect

can be seen in Ref. 13, where the coefficient of the nonlinear term of the model depends on the neutron fluence linearly, and the slope becomes lower at higher dose rates. We will continue develop the multiscale method in the main text to allow quantitative treatment of the irradiation dose and dose rate in first-principles calculations, and study the mechanism of these dose rate effects in the future.

## V. CALCULATION DETAILS

### A. Geant4

In Geant4 simulations, we do not use the actual dimensions of transistors and the actual number of $\gamma$ photons corresponding to the experimental dose due to the following considerations. (1) The size of an actual transistor is too small that most of the $\gamma$ photons would pass through with no interaction, so a very large number of $\gamma$ photons are needed in the simulation to reach the doses used in experiments. (2) The computational cost of the simulation increased significantly as we turned off the energy cutoff. (3) As there are no previous work that simulates the effect of $\gamma$-ray irradiation by combining Monte-Carlo and excited-state first-principles calculations, this work is more of a proof of concept for checking the validity of the method before constructing a realistic model. Therefore we setup the calculation using as few $\gamma$ photons as possible.

A 10 cm×10 cm×10 cm bulk Silicon system is used in Geant4. Its top plane is set as the $\gamma$-ray source, and the $\gamma$ photons are all in the -z direction. These settings reduce the computational cost as the $\gamma$ photon is always absorbed. The experiments in Refs. [13, 17, 18] use a Co-60 $\gamma$-ray source which has two main peaks (1173.2 keV and 1332.5 keV) with similar heights. We set the $\gamma$-ray source according to this in simulation, and it generates two $\gamma$ photons correspondingly in each simulation.

The agglomerative hierarchical clustering (AHC) analysis is carried out as follows. We first prepare the analysis by running AHC with single linkage[19] and $L^2$ norm to find all electron groups whose shortest distances to neighbors are larger than 1 $\mu$m. The actual analysis is done on these groups. For the actual analysis, we carry out AHC with complete linkage[19] on a group to find all the clusters that can fit in a $3 \times 3 \times 3$ supercell. The analysis is done twice with $L^2$ norm (a sphere with the same volume as the supercell) and $L^\infty$ norm (a supercell aligned with the x,y,z axes of the system) respectively, and they yield similar results. We use this procedure to reduce the high computational cost of AHC with complete linkage.

### B. DFT

We use the following parameters for the ground-state DFT and ΔSCF calculations in VASP. We use the projector augmented waves (PAW) generated using the PBE functional. The energy cutoff for PAWs is set to 400 eV for all calculations, which is equal to the maximum cutoff of O as listed in the pseudopotential file. The energy convergence criterion for SCF is set to $10^{-6}$ eV for geometry optimization and NEB, and $10^{-8}$ eV for the calculation of Vineyard prefactor. The force convergence criterion is set to 0.001 eV/Åfor geometry optimizations and 0.01 eV/Åfor NEB.

We checked the effect of dipole corrections on the calculations of charged $V_2$. The correction to the energies can be as large as several eV, but the NEB curve is only changed by about $10^{-2}$ eV since it only depends on the relative magnitude of the energies. Therefore we do not include the dipole correction in the results of the main text.

We use the following parameters for the dynamics simulations in PWmat. We use the SG15 norm-conserving pseudopotential[20]. The plane wave energy cutoff is set to 60 Ryd. A total of 510 bands are calculated in TDDFT, and the first 466 bands are propagated by expansion on the basis set formed by the Kohn-Sham orbitals 1 to 500. The time step for TDDFT is 0.1 fs. We cannot directly set the ΔSCF occupation numbers, since the occupation numbers are unchanged in TDDFT and only the orbitals are propagated in time. Instead, we manually set the linear combination coefficients at the initial time to achieve the same effect, since the propagated orbitals are represented by linear combination of Kohn-Sham orbitals at the current time. The dephasing times for the Boltzmann factor method are estimated according to the change of orbital energies with respect to time[21–24], and the average value for all states is in $2 \sim 3$ fs from an microcanonical (NVE) simulation of a $V_2$ defect. We use a 2.5 fs dephasing time in all simulations with the Boltzmann factor for most of the bands. The dephasing time of the last 5 bands are set to 0.0001 fs as recommended.[22]

$N_{\mathrm{exc}}$ at a specific time is calculated using the ground-state KS orbitals at that time. We first calculate the ground-state KS occupation numbers at that time, and then obtain the excited-state KS occupation numbers as the sums of overlaps between the time-dependent orbitals and the ground-state KS orbitals, and $N_{\mathrm{exc}}$ can then be obtained from the difference between the excited-state and ground-state occupation numbers.

[1] A. T. B. Gilbert, N. A. Besley, and P. M. W. Gill. Self-consistent field calculations of excited states using the maximum overlap method (MOM). *J. Phys. Chem. A*, 112:13164, 2008.

[2] Y. C. Park, M. Krykunov, and T. Ziegler. On the relation between adiabatic time dependent density functional theory (tddft) and the $\delta$scf-dft method. introducing a numerically stable $\delta$scf-dft scheme for local functionals based on constricted variational dft. *Mol. Phys.*, 113:1636, 2015.

[3] D. Hait and M. Head-Gordon. Excited state orbital optimization via minimizing the square of the gradient: General approach and application to singly and doubly excited states via density functional theory. *J. Chem. Theory Comput.*, 16:1699, 2020.

[4] H. Bracht, E. E. Haller, and R. Clark-Phelps. Silicon self-diffusion in isotope heterostructures. *Phys. Rev. Lett.*, 81:393, 1998.

[5] G. Vineyard. Frequency factors and isotope effects in solid state rate processes. *J. Phys. Chem. Solids*, 3:121, 1957.

[6] L. Kong and L. Lewis. Transition state theory of the preexponential factors for self-diffusion on cu, ag, and ni surfaces. *Phys. Rev. B*, 74:073412, 2006.

[7] M. Mikelsen, E. V. Monakhov, G. Alfieri, B. S. Avset, and B. G. Svensson. Kinetics of divacancy annealing and divacancy-oxygen formation in oxygen-enriched high-purity silicon. *Phys. Rev. B*, 72:195207, 2005.

[8] A. Endrös. Properties of hydrogen, oxygen and carbon in si. *Solid State Phenom.*, 32-33:143, 1993.

[9] A. Hallén, N. Keskitalo, L. Josyula, and B. G. Svensson. Migration energy for the silicon self-interstitial. *J. Appl. Phys.*, 86:214, 1999.

[10] T. Lazauskas, S. D. Kenny, and R. Smith. Influence of the prefactor to defect motion in $\alpha$-iron during long time scale simulations. *J. Phys.: Condens. Matter*, 26:395007, 2014.

[11] Q. Gibaru, C. Inguimbert, P. Caron, M. Raine, D. Lambert, and J. Puech. Geant4 physics processes for microdosimetry and secondary electron emission simulation: Extension of microelec to very low energies and 11 materials (c, al, si, ti, ni, cu, ge, ag, w, kapton and sio2). *Nucl. Instrum. Methods Phys. Res. B*, 487:66, 2021.

[12] R. D. Narayan, R. Miranda, and P. Rez. Monte carlo simulation for the electron cascade due to gamma rays in semiconductor radiation detectors. *J. Appl. Phys.*, 111:064910, 2012.

[13] Y. Song and S.-H. Wei. Origin of irradiation synergistic effects in silicon bipolar transistors. *ACS Appl. Electron. Mater.*, 2:3783, 2020.

[14] R. A. Casali, H. Rücker, and M. Methfessel. Interaction of vacancies with interstitial oxygen in silicon. *Appl. Phys. Lett.*, 78:913, 2001.

[15] T. R. Waite. General theory of bimolecular reaction rates in solids and liquids. *J. Chem. Phys.*, 28:103, 1958.

[16] K. Wu, J. Li, D. Zou, Y. Lu, J. Feng, X. Lv, D. Qiu, X. Fan, X. Xu, and J. Wu. Neutron flux effects in silicon based bipolar junction transistors. *Nucl. Instrum. Methods Phys. Res. A*, 913:85, 2019.

[17] Y. Song, Y. Zhang, Y. Liu, J. Zhao, D. Meng, H. Zhou, X. Wang, M. Lan, and S.-H. Wei. Mechanism of synergistic effects of neutron- and gamma-ray-radiated pnp bipolar transistors. *ACS Appl. Electron. Mater.*, 1:538, 2019.

[18] Y. Song, H. Zhou, X.-F. Cai, Y. Liu, P. Yang, G.-H. Zhang, Y. Zhang, M. Lan, and S.-H. Wei. Defect dynamic model of the synergistic effect in neutron-and $\gamma$-ray-irradiated silicon npn transistors. *ACS Appl. Mater. Interfaces*, 12:29993, 2020.

[19] S. Bochkanov. ALGLIB (www.alglib.net).

[20] M. Schlipf and F. Gygi. Optimization algorithm for the generation of oncv pseudopotentials. *Comput. Phys. Comm.*, 196:36, 2015.

[21] L-.W. Wang. Natural orbital branching scheme for time-dependent density functional theory nonadiabatic simulations. *J. Phys. Chem. A*, 124:9075, 2020.

[22] 2022. PWmat user manual (www.pwmat.com/pwmat-resource/Manual.pdf).

[23] W.-H. Liu, J.-W. Luo, S.-S. Li, and L.-W. Wang. The critical role of hot carrier cooling in optically excited structural transitions. *NPJ Comput. Mater.*, 7:117, 2021.

[24] J. Kang and L.-W. Wang. Nonadiabatic molecular dynamics with decoherence and detailed balance under a density matrix ensemble formalism. *Phys. Rev. B*, 99:224303, 2019.
